# Supplementary material for: Implications of the multi-minima character of molecular crystal phases onto the free energy
Source: arXiv:2501.18372 source file (2025-01-30)
Supplement: Supplementary file 1 [file molecular_crystals_physical_review_supplementary_information.pdf]

# Supplementary information to "Implications of the multi-minima character of molecular crystal phases onto the free energy"

Marco Krummenacher, Martin Sommer-Jörgendsen, Moritz Gubler, Jonas A. Finkler, Ehsan Rahmatizad Khajehpasha, Giuseppe Fisicaro and Stefan Goedecker

July 2024

## 1 Machine Learned Potential

In Fig. a correlation plot of the NequIP machine learned potential is given. The errors for the energies are 15.8 meV per atom in the training set and 17.8 meV per atom for the test set respectively. The training set consists of 16'000 structures while the validation set consists of 30'000 structures. The evaluation of the forces results in an error of 98 meV/Åfor the training set and 109 meV/Åfor the test set respectively.

## 2 Structures

In the following the coordinates of the 10 lowest structures found with the minima hopping are given.

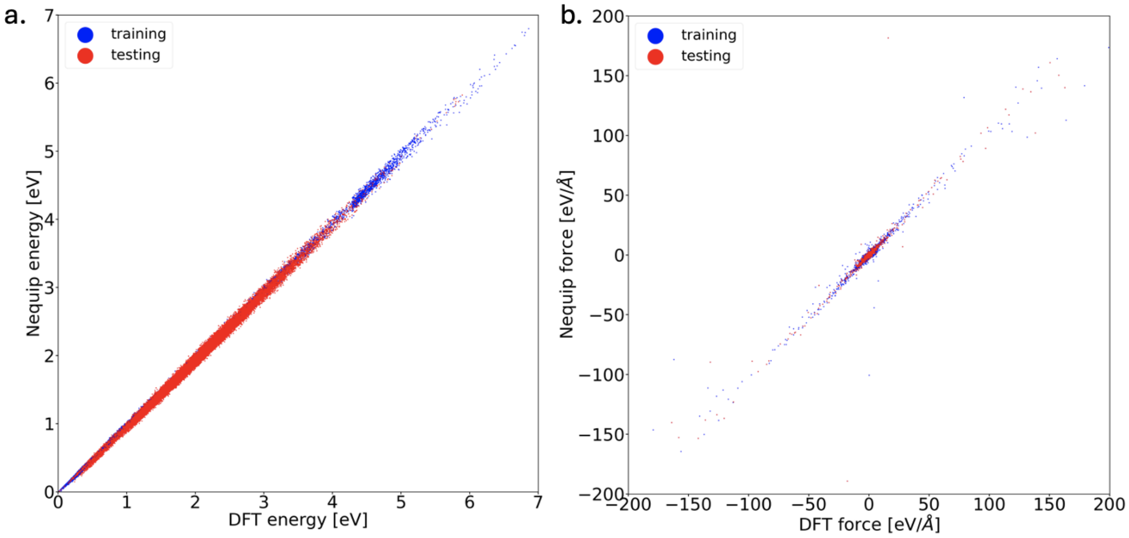


Figure 1: Accuracy of the machine learned energies and forces: Panel a): NequiP energies vs DFT energies, panel b): NequiP forces vs DFT forces

| | | | |
|---|---|---|---|
| $X_{Lattice}$ | 3.34767409 | 0.12362053 | -0.2413044 |
| $Y_{Lattice}$ | 0.85477409 | 13.9820356 | -0.1209118 |
| $Z_{Lattice}$ | 0.49036186 | 3.45784418 | 11.5747239 |
| C | 1.41691574 | 1.84374183 | 5.31242779 |
| C | 4.17259443 | 8.80704754 | 5.99334462 |
| H | 1.09264028 | 2.85423171 | 5.00085696 |
| H | 4.00782423 | 7.76576639 | 6.32779945 |
| N | 1.93093217 | 1.63127229 | 6.47439858 |
| N | 4.46300062 | 9.08208841 | 4.76923736 |
| C | 0.82926308 | -1.18578969 | 2.35222841 |
| C | 3.62689847 | 11.71337603 | 9.07891906 |
| C | 2.52028075 | 4.76776128 | 9.25816944 |
| C | 4.88965837 | 6.04652336 | 1.84987485 |
| C | 1.26444913 | -1.52840571 | 3.64308067 |
| C | 3.91179524 | 12.12051749 | 7.76254471 |
| C | 2.62746294 | 5.02061682 | 7.88609932 |
| C | 5.20040719 | 5.77794806 | 3.18759159 |
| C | 1.45807370 | -0.55474085 | 4.61036767 |
| C | 4.10456433 | 11.18917802 | 6.75509280 |
| C | 2.44440993 | 4.01196367 | 6.95050785 |
| C | 5.07105611 | 6.75268204 | 4.16614847 |
| C | 1.21717521 | 0.79666647 | 4.32112769 |
| C | 4.01668896 | 9.81511927 | 7.02978564 |
| C | 2.13277520 | 2.70200347 | 7.35778879 |
| C | 4.61702068 | 8.04322991 | 3.83880649 |
| C | 0.75942938 | 1.13770975 | 3.03887961 |
| C | 3.72898378 | 9.40788403 | 8.34115314 |
| C | 2.06513767 | 2.43913006 | 8.73260754 |
| C | 4.33496012 | 8.32337096 | 2.49525324 |
| C | 0.57687633 | 0.16151092 | 2.06722453 |
| C | 3.53908695 | 10.34477490 | 9.35018543 |
| C | 2.24395128 | 3.45659302 | 9.66021630 |
| C | 4.45906978 | 7.33726030 | 1.52479744 |
| C | 0.61538885 | -2.24543529 | 1.30737329 |
| C | 3.44957757 | 12.72814278 | 10.17069624 |
| C | 2.72149459 | 5.86536673 | 10.26463624 |
| C | 5.03810429 | 4.98379246 | 0.79847121 |
| H | 1.44801301 | -2.57610824 | 3.88888993 |
| H | 3.96455625 | 13.18587413 | 7.52756581 |
| H | 2.87454654 | 6.02838297 | 7.54798399 |
| H | 5.56355408 | 4.78554976 | 3.45995974 |
| H | 1.79233887 | -0.81895663 | 5.61021703 |
| H | 4.31397176 | 11.50244787 | 5.73500064 |
| H | 2.56796152 | 4.23040648 | 5.89161769 |
| H | 5.33945336 | 6.52161994 | 5.19483371 |
| H | 0.55198739 | 2.18456165 | 2.80919123 |
| H | 3.64684401 | 8.34226917 | 8.56175566 |
| H | 1.84055636 | 1.42370167 | 9.05086026 |
| H | 3.99027176 | 9.32297390 | 2.23965608 |
| H | 0.22682254 | 0.44421844 | 1.07421855 |
| H | 3.29742967 | 10.01442634 | 10.35975967 |
| H | 2.16797108 | 3.23562616 | 10.72513396 |
| H | 4.21459825 | 7.56908151 | 0.48884432 |
| H | 0.93824254 | -1.92093364 | 0.30946390 |
| H | 2.83223542 | 13.57152257 | 9.83766176 |
| H | 2.21419673 | 6.79406331 | 9.96881419 |
| H | 6.09827704 | 4.82315617 | 0.54261900 |
| H | 1.12819886 | -3.18031188 | 1.56341088 |
| H | 2.99408450 | 12.29088941 | 11.06727517 |
| H | 3.78919269 | 6.11966913 | 10.36986323 |
| H | 4.52649453 | 5.25290970 | -0.13367113 |
| H | -0.45649667 | -2.48792621 | 1.21500433 |
| H | 4.41773653 | 13.15427945 | 10.47300498 |
| H | 2.36690856 | 5.57589540 | 11.26166338 |
| H | 4.65832355 | 4.01076079 | 1.13932117 |

Table 1: Coordinates of a structure of Form III with a potential energy of -6112.940506 eV

| | | | |
|---|---|---|---|
| $X_{Lattice}$ | 3.345975454 | 0.087376796 | -0.3725080 |
| $Y_{Lattice}$ | 0.035247089 | 13.13916165 | 1.68116960 |
| $Z_{Lattice}$ | -2.54615097 | 1.534420746 | 13.1659515 |
| C | -0.63481783 | 13.96205844 | 8.71388803 |
| C | 1.47974829 | 6.75818398 | 6.69646520 |
| H | -0.92316209 | 12.91074884 | 8.88905272 |
| H | 1.86272492 | 5.97077193 | 7.36952898 |
| N | -0.38329157 | 14.39552792 | 7.52718975 |
| N | 1.40411834 | 7.99108760 | 7.05880312 |
| C | -0.43512843 | 16.32887181 | 12.27491341 |
| C | 0.21982034 | 5.32212956 | 2.87218030 |
| C | -0.51807837 | 11.69692019 | 4.26628867 |
| C | 2.32645135 | 9.36750206 | 10.95432421 |
| C | -0.21245712 | 16.91097420 | 11.01826324 |
| C | 0.62399086 | 4.44259349 | 3.87978268 |
| C | -0.04232808 | 11.27161774 | 5.51422118 |
| C | 2.41757171 | 10.19136663 | 9.82630626 |
| C | -0.26784123 | 16.15975374 | 9.85536003 |
| C | 1.05081344 | 4.91975393 | 5.11177524 |
| C | 0.01670226 | 12.14858659 | 6.58781167 |
| C | 2.12248048 | 9.71161059 | 8.55951666 |
| C | -0.56139214 | 14.78933738 | 9.91118746 |
| C | 1.05610116 | 6.29399152 | 5.38519924 |
| C | -0.40696960 | 13.48300223 | 6.45940236 |
| C | 1.74090591 | 8.37453852 | 8.36340865 |
| C | -0.78677758 | 14.20240817 | 11.16750485 |
| C | 0.63716847 | 7.18043188 | 4.37886025 |
| C | -0.83980664 | 13.92279757 | 5.20017601 |
| C | 1.66248758 | 7.53860920 | 9.48950855 |
| C | -0.71650299 | 14.95814485 | 12.33000613 |
| C | 0.23096815 | 6.69927510 | 3.14512259 |
| C | -0.90727554 | 13.03559016 | 4.13220462 |
| C | 1.94940041 | 8.03363023 | 10.75594868 |
| C | -0.39907962 | 17.15831963 | 13.52647747 |
| C | -0.20195569 | 4.80114987 | 1.52709026 |
| C | -0.56791802 | 10.74681877 | 3.10053355 |
| C | 2.61374197 | 9.90999571 | 12.32789312 |
| H | 0.01076095 | 17.97645070 | 10.96344982 |
| H | 0.61857139 | 3.36791832 | 3.70297402 |
| H | 0.29057501 | 10.24210572 | 5.65804409 |
| H | 2.72139715 | 11.23144501 | 9.94822281 |
| H | -0.08254783 | 16.61204852 | 8.88437453 |
| H | 1.38540743 | 4.21178222 | 5.86766714 |
| H | 0.41863106 | 11.80379506 | 7.53874268 |
| H | 2.18225533 | 10.35466632 | 7.68437701 |
| H | -1.02156698 | 13.13905775 | 11.22420423 |
| H | 0.64525797 | 8.24742696 | 4.59193382 |
| H | -1.15413019 | 14.95856084 | 5.08808107 |
| H | 1.33051501 | 6.50794359 | 9.38113442 |
| H | -0.89303945 | 14.48420865 | 13.29619545 |
| H | -0.07778688 | 7.40095506 | 2.37005944 |
| H | -1.28191502 | 13.38624560 | 3.16941235 |
| H | 1.85637345 | 7.37238903 | 11.61776443 |
| H | 0.17410733 | 16.67209846 | 14.32810419 |
| H | -1.29716100 | 4.68874641 | 1.47066124 |
| H | -1.13869481 | 11.15990094 | 2.25853844 |
| H | 3.69645202 | 10.05627108 | 12.47577025 |
| H | 0.01593396 | 18.15717481 | 13.34553804 |
| H | 0.07622639 | 5.48244129 | 0.71298573 |
| H | -1.00439900 | 9.77731702 | 3.37958694 |
| H | 2.27362728 | 9.23286812 | 13.12107319 |
| H | -1.41699692 | 17.30397373 | 13.92399513 |
| H | 0.22308579 | 3.81009186 | 1.32425515 |
| H | 0.44569787 | 10.53101377 | 2.72533036 |
| H | 2.14904015 | 10.89362743 | 12.48868342 |

Table 2: Coordinates of a structure of Form II with a potential energy of -6112.876479 eV

| | | | |
|---|---|---|---|
| $X_{Lattice}$ | 3.34507737 | -0.2676107 | 0.290385295 |
| $Y_{Lattice}$ | -0.4048623 | 12.3262479 | -1.11000095 |
| $Z_{Lattice}$ | 1.93381158 | 4.38102550 | 13.06224428 |
| C | 0.40701488 | 5.79596683 | -0.27179532 |
| C | 3.69501049 | 8.63289037 | 5.94446258 |
| H | 0.57636837 | 5.85501421 | 0.81856335 |
| H | 3.55323906 | 8.70047590 | 4.85044881 |
| N | 0.06730906 | 6.83529624 | -0.95233834 |
| N | 3.45448209 | 7.54978599 | 6.59926778 |
| C | 1.11086111 | 1.90983087 | -1.91555137 |
| C | 5.07550960 | 12.28693085 | 7.69492885 |
| C | -0.48453827 | 10.60662777 | 0.89670156 |
| C | 2.26379289 | 3.91337367 | 4.77048990 |
| C | 0.87998735 | 3.01038878 | -2.76051414 |
| C | 4.77442968 | 11.18304450 | 8.50918313 |
| C | -0.76862598 | 9.43350618 | 1.60560395 |
| C | 2.83131716 | 4.93531039 | 3.99619417 |
| C | 0.62882193 | 4.27049754 | -2.24147432 |
| C | 4.33692393 | 9.98866184 | 7.95420055 |
| C | -0.60309566 | 8.18280162 | 1.02498379 |
| C | 3.23336246 | 6.14089279 | 4.55421371 |
| C | 0.61826221 | 4.48008317 | -0.85452638 |
| C | 4.17160251 | 9.85839951 | 6.56560141 |
| C | -0.13435108 | 8.05965147 | -0.29563573 |
| C | 3.06315515 | 6.37991283 | 5.92913926 |
| C | 0.86929876 | 3.38792453 | -0.01038389 |
| C | 4.48182728 | 10.95791548 | 5.75235060 |
| C | 0.10927282 | 9.23372646 | -1.01919096 |
| C | 2.49350340 | 5.35782873 | 6.70479930 |
| C | 1.10329322 | 2.12127061 | -0.53362263 |
| C | 4.94580300 | 12.14468014 | 6.30931456 |
| C | -0.05406810 | 10.47967951 | -0.42826176 |
| C | 2.09812304 | 4.15242032 | 6.13705562 |
| C | 1.32755761 | 0.53819826 | -2.48842200 |
| C | 5.48757972 | 13.60064905 | 8.29311544 |
| C | -0.66018291 | 11.95833638 | 1.53183279 |
| C | 1.90877416 | 2.59172579 | 4.15344839 |
| H | 0.91576843 | 2.87880693 | -3.84415212 |
| H | 4.88041394 | 11.26497204 | 9.59321974 |
| H | -1.13622616 | 9.50250493 | 2.63060290 |
| H | 2.97526778 | 4.76712634 | 2.92715666 |
| H | 0.46266840 | 5.12107706 | -2.89753719 |
| H | 4.12423734 | 9.12880193 | 8.58436404 |
| H | -0.86331350 | 7.29099193 | 1.59293348 |
| H | 3.70586841 | 6.88797792 | 3.91905354 |
| H | 0.88381739 | 3.54351388 | 1.06989888 |
| H | 4.36773497 | 10.86909244 | 4.67122512 |
| H | 0.45302642 | 9.14209565 | -2.04678748 |
| H | 2.35575107 | 5.54207696 | 7.76813088 |
| H | 1.30836365 | 1.28771918 | 0.13810317 |
| H | 5.20011427 | 12.98324562 | 5.66148407 |
| H | 0.15856068 | 11.37853744 | -1.00745581 |
| H | 1.64846047 | 3.38438249 | 6.76615209 |
| H | 1.80127030 | -0.13622085 | -1.76428961 |
| H | 4.60780468 | 14.22068253 | 8.52355464 |
| H | -0.31105982 | 11.97530681 | 2.57362424 |
| H | 1.48044695 | 2.71075629 | 3.14930545 |
| H | 0.37003541 | 0.07850191 | -2.77561505 |
| H | 6.02977955 | 13.46070569 | 9.23511106 |
| H | -1.72258464 | 12.25036211 | 1.56023130 |
| H | 1.19343219 | 2.03475656 | 4.77034002 |
| H | 1.94168709 | 0.57095512 | -3.39781150 |
| H | 6.11588988 | 14.18304941 | 7.60735426 |
| H | -0.13571259 | 12.74445361 | 0.97408863 |
| H | 2.79876924 | 1.95613631 | 4.03970944 |

Table 3: Coordinates of a structure of Form I with a potential energy of -6112.853695 eV

| | | | |
|---|---|---|---|
| $X_{Lattice}$ | 3.342688307 | -0.38021173 | -0.1172943 |
| $Y_{Lattice}$ | -2.70869107 | 12.528986055 | 1.073768499 |
| $Z_{Lattice}$ | -2.47788249 | -2.004671143 | 13.44372647 |
| C | -0.03210523 | -0.71350042 | 6.63747514 |
| C | -0.33648738 | 4.46129232 | 7.41839218 |
| H | 0.36628295 | -0.08426983 | 7.45389172 |
| H | -0.77576940 | 3.71543932 | 6.73049147 |
| N | -0.63457909 | -1.82481568 | 6.88004667 |
| N | -0.17095447 | 5.68887463 | 7.07194283 |
| C | 0.49878100 | 0.93154515 | 2.72632898 |
| C | 0.67727987 | 2.86908003 | 11.26199906 |
| C | -1.23998396 | -3.12844069 | 10.85981612 |
| C | -0.87248646 | 7.08084686 | 3.14159406 |
| C | 0.82166577 | 1.66862411 | 3.86888908 |
| C | 0.16269581 | 2.05363461 | 10.24649434 |
| C | -1.04211762 | -4.02756122 | 9.80640902 |
| C | -0.96925761 | 7.92507860 | 4.25373514 |
| C | 0.66132602 | 1.11926328 | 5.13588266 |
| C | -0.16857272 | 2.58194801 | 9.00535225 |
| C | -0.85894095 | -3.59541564 | 8.49821115 |
| C | -0.74987257 | 7.45470177 | 5.54077906 |
| C | 0.16390069 | -0.18191164 | 5.29571071 |
| C | 0.03216252 | 3.94200131 | 8.72846919 |
| C | -0.84086159 | -2.22383454 | 8.21005721 |
| C | -0.45059755 | 6.09809162 | 5.75956584 |
| C | -0.12642628 | -0.93690968 | 4.14927007 |
| C | 0.59291458 | 4.75283989 | 9.73001313 |
| C | -1.07984985 | -1.31620944 | 9.25813145 |
| C | -0.37639112 | 5.24100196 | 4.64913933 |
| C | 0.03999429 | -0.38656727 | 2.88921847 |
| C | 0.89277539 | 4.22516229 | 10.97825490 |
| C | -1.27044693 | -1.76273444 | 10.55818433 |
| C | -0.57729474 | 5.73041221 | 3.36461691 |
| C | 0.59509306 | 1.55171192 | 1.36253591 |
| C | 0.95316470 | 2.29330704 | 12.62063758 |
| C | -1.44498027 | -3.62114700 | 12.26520107 |
| C | -1.04303674 | 7.63297902 | 1.75347435 |
| H | 1.20453696 | 2.68325348 | 3.76067392 |
| H | 0.01519646 | 0.99095344 | 10.44175688 |
| H | -1.03200957 | -5.09660374 | 10.01934952 |
| H | -1.21140728 | 8.97730568 | 4.10241550 |
| H | 0.91171864 | 1.70689233 | 6.02091949 |
| H | -0.59284383 | 1.93993119 | 8.23214060 |
| H | -0.70832770 | -4.31278484 | 7.69131050 |
| H | -0.79545754 | 8.13349457 | 6.39187180 |
| H | -0.47450095 | -1.95810635 | 4.27916901 |
| H | 0.79534099 | 5.79669776 | 9.49894428 |
| H | -1.14943637 | -0.25232125 | 9.03908840 |
| H | -0.09626558 | 4.19887554 | 4.78644671 |
| H | -0.19256123 | -0.98414836 | 2.00560350 |
| H | 1.31796388 | 4.87139043 | 11.74763008 |
| H | -1.46333085 | -1.03855415 | 11.35184995 |
| H | -0.46743345 | 5.05726480 | 2.51198105 |
| H | -0.40380120 | 1.84564921 | 1.00312178 |
| H | 1.63305714 | 2.92424937 | 13.20474506 |
| H | -2.50163601 | -3.53635427 | 12.56748810 |
| H | -2.09733161 | 7.88174197 | 1.55002658 |
| H | 1.20951597 | 2.46061555 | 1.37242190 |
| H | 0.02317714 | 2.19787851 | 13.20195740 |
| H | -0.86779038 | -3.04158953 | 13.00004236 |
| H | -0.72432204 | 6.92275366 | 0.98104893 |
| H | 0.99726137 | 0.85503477 | 0.61540903 |
| H | 1.38024741 | 1.28479451 | 12.54918703 |
| H | -1.16874079 | -4.67711908 | 12.36522620 |
| H | -0.47827891 | 8.56608049 | 1.61912121 |

Table 4: Coordinates of a structure of Form II with a potential energy of -6112.833329 eV

| | | | |
|---|---|---|---|
| $X_{Lattice}$ | 3.36966918 | 0.088449424 | -0.1063182 |
| $Y_{Lattice}$ | 1.37397286 | 13.58617344 | -0.420258764 |
| $Z_{Lattice}$ | 0.24822109 | 1.227417239 | 11.97013883 |
| C | 2.80980175 | 6.97778079 | 0.11292911 |
| C | 2.38864351 | 7.10465120 | 5.26145983 |
| H | 3.16374805 | 6.30313853 | 0.91223870 |
| H | 1.96738356 | 7.61613877 | 4.37662181 |
| N | 2.25112093 | 6.52063280 | -0.95280309 |
| N | 2.47016538 | 7.68320399 | 6.40764954 |
| C | 3.37009642 | 11.13311280 | 0.96003119 |
| C | 3.53026011 | 3.05537197 | 4.46868201 |
| C | 1.45842454 | 2.39364454 | -1.48040835 |
| C | 1.35104660 | 11.72603932 | 6.99260423 |
| C | 3.59880036 | 10.15866634 | 1.93686130 |
| C | 3.08670728 | 3.90295533 | 3.44810908 |
| C | 1.72114587 | 3.24627484 | -2.55953356 |
| C | 1.37140089 | 10.80093703 | 8.03964859 |
| C | 3.43484018 | 8.81069725 | 1.64384317 |
| C | 2.72456084 | 5.21680441 | 3.72040238 |
| C | 1.98555825 | 4.59829125 | -2.37718805 |
| C | 1.74495792 | 9.47715817 | 7.83314251 |
| C | 3.01168710 | 8.39712234 | 0.37078775 |
| C | 2.82155794 | 5.73562003 | 5.01809201 |
| C | 2.01653719 | 5.14212628 | -1.08486274 |
| C | 2.08881880 | 9.02688378 | 6.54890282 |
| C | 2.79773973 | 9.37059550 | -0.61480517 |
| C | 3.31525620 | 4.90051294 | 6.03628017 |
| C | 1.73240956 | 4.29587333 | 0.00133363 |
| C | 2.07392006 | 9.95351113 | 5.49164969 |
| C | 2.97983543 | 10.71355917 | -0.32153186 |
| C | 3.64607076 | 3.58144878 | 5.76457957 |
| C | 1.45880322 | 2.94777960 | -0.19688415 |
| C | 1.70811338 | 11.27400014 | 5.71445200 |
| C | 3.55327712 | 12.58974176 | 1.28579529 |
| C | 3.85321211 | 1.61489909 | 4.18043692 |
| C | 1.19161459 | 0.93238424 | -1.70200741 |
| C | 1.01696900 | 13.16889295 | 7.24341620 |
| H | 3.90890752 | 10.46254227 | 2.93652992 |
| H | 2.99875034 | 3.51649645 | 2.43220218 |
| H | 1.70683548 | 2.84082899 | -3.57183233 |
| H | 1.09393669 | 11.12610514 | 9.04214335 |
| H | 3.62048633 | 8.05965122 | 2.41378718 |
| H | 2.33946380 | 5.85463395 | 2.92440001 |
| H | 2.16825177 | 5.25035096 | -3.23190916 |
| H | 1.76900039 | 8.77489946 | 8.66642775 |
| H | 2.49367526 | 9.04628831 | -1.60660551 |
| H | 3.42473230 | 5.31022321 | 7.03810761 |
| H | 1.67286742 | 4.70902006 | 1.00680358 |
| H | 2.38338335 | 9.64834541 | 4.49403743 |
| H | 2.80622067 | 11.46192914 | -1.09690550 |
| H | 3.99992052 | 2.93849042 | 6.57195414 |
| H | 1.21570289 | 2.31899009 | 0.66172332 |
| H | 1.72002181 | 11.97820404 | 4.87934001 |
| H | 3.16584224 | 12.83549243 | 2.28366018 |
| H | 4.94183844 | 1.44611403 | 4.15916189 |
| H | 2.12963784 | 0.36097750 | -1.77384593 |
| H | 0.38514247 | 13.58883326 | 6.44901896 |
| H | 4.62359130 | 12.85487169 | 1.29703156 |
| H | 3.45690825 | 0.94244504 | 4.95246380 |
| H | 0.64162045 | 0.75952256 | -2.63632209 |
| H | 1.92650226 | 13.78734927 | 7.28634086 |
| H | 3.07519058 | 13.24512763 | 0.54786507 |
| H | 3.46213386 | 1.29998107 | 3.20511789 |
| H | 0.61098696 | 0.49733376 | -0.87878859 |
| H | 0.49494132 | 13.29700533 | 8.19938186 |

Table 5: Coordinates of a structure of Form II with a potential energy of -6112.829774 eV

| | | | |
|---|---|---|---|
| $X_{Lattice}$ | 3.37310393 | -0.0868030 | -0.0168310 |
| $Y_{Lattice}$ | 2.23829702 | 13.94587217 | -1.6434731 |
| $Z_{Lattice}$ | 0.12363888 | 1.31962977 | 11.783698 |
| C | 2.28800373 | 6.63838696 | -0.53706823 |
| C | 2.23108875 | 7.95492495 | 5.50095897 |
| H | 2.63091541 | 6.84512380 | 0.49223847 |
| H | 2.42398207 | 7.40899516 | 6.44209066 |
| N | 1.77052711 | 7.55497884 | -1.27805669 |
| N | 1.76534669 | 7.36492955 | 4.45559056 |
| C | 2.69883909 | 2.55636671 | -1.75744942 |
| C | 3.21013893 | 12.11326816 | 5.64762763 |
| C | 1.16076222 | 11.53815627 | 0.01683698 |
| C | 0.91284426 | 3.21947190 | 4.36641048 |
| C | 2.33640507 | 3.54429045 | -2.68687816 |
| C | 3.24199864 | 11.32295745 | 6.79791530 |
| C | 1.13340035 | 10.49371219 | 0.94853836 |
| C | 1.26961928 | 3.93775117 | 3.21867965 |
| C | 2.20144825 | 4.87187186 | -2.31134912 |
| C | 2.92708750 | 9.96916598 | 6.74631715 |
| C | 1.34492749 | 9.17330665 | 0.56965687 |
| C | 1.52666026 | 5.29954583 | 3.27428836 |
| C | 2.44495666 | 5.25929304 | -0.98523677 |
| C | 2.55762737 | 9.37265611 | 5.53237299 |
| C | 1.57526535 | 8.85319209 | -0.78027750 |
| C | 1.46876314 | 5.99467269 | 4.49010683 |
| C | 2.84648616 | 4.28049423 | -0.06273163 |
| C | 2.54312668 | 10.15785649 | 4.36883498 |
| C | 1.55286802 | 9.89168115 | -1.71997318 |
| C | 1.07858344 | 5.28444322 | 5.63922642 |
| C | 2.95398507 | 2.94753577 | -0.43910645 |
| C | 2.86796095 | 11.50342907 | 4.42895869 |
| C | 1.36864023 | 11.20999032 | -1.32606922 |
| C | 0.80975052 | 3.92203602 | 5.57153162 |
| C | 2.82235104 | 1.11659690 | -2.17343036 |
| C | 3.50138122 | 13.58322725 | 5.72695270 |
| C | 0.95213218 | 12.96282206 | 0.45244988 |
| C | 0.66661470 | 1.74113126 | 4.29168566 |
| H | 2.14708721 | 3.25374837 | -3.72049831 |
| H | 3.51794758 | 11.77630175 | 7.74921226 |
| H | 0.94255399 | 10.72064637 | 1.99725713 |
| H | 1.34032168 | 3.41701726 | 2.26253871 |
| H | 1.89667256 | 5.63490313 | -3.02588151 |
| H | 2.95765251 | 9.36871657 | 7.65833517 |
| H | 1.30498486 | 8.39147740 | 1.32897453 |
| H | 1.79213705 | 5.85944584 | 2.37958395 |
| H | 3.06048185 | 4.57335137 | 0.96459760 |
| H | 2.29194930 | 9.67867949 | 3.42559244 |
| H | 1.69560270 | 9.63440697 | -2.76544414 |
| H | 0.95063162 | 5.80937325 | 6.58527250 |
| H | 3.24685529 | 2.19879607 | 0.29876021 |
| H | 2.85880791 | 12.10141686 | 3.51545317 |
| H | 1.38710874 | 12.00276704 | -2.07730289 |
| H | 0.49394139 | 3.39395887 | 6.47289143 |
| H | 2.37016237 | 0.93662899 | -3.15689104 |
| H | 4.06939991 | 13.93649448 | 4.85705730 |
| H | 1.38796067 | 13.67919224 | -0.25787835 |
| H | 0.09519417 | 1.37881097 | 5.15437309 |
| H | 3.88030197 | 0.81692263 | -2.24802304 |
| H | 2.56881141 | 14.16727428 | 5.75128784 |
| H | 1.38001006 | 13.15157819 | 1.44642820 |
| H | 1.61538876 | 1.18348209 | 4.27777184 |
| H | 2.36139985 | 0.43514768 | -1.44380685 |
| H | 4.05790027 | 13.83113605 | 6.63885653 |
| H | -0.12059721 | 13.20538695 | 0.52598831 |
| H | 0.12995789 | 1.46564008 | 3.37436101 |

Table 6: Coordinates of a structure of Form II with a potential energy of -6112.804417 eV

| | | | |
|---|---|---|---|
| $X_{Lattice}$ | 3.37985083 | 0.0915646478 | -0.151758 |
| $Y_{Lattice}$ | -0.1268543 | 12.340592255 | 1.4951694 |
| $Z_{Lattice}$ | -1.0064070 | 0.034888722 | 13.312571 |
| C | 1.83038201 | 12.12373695 | 8.58838820 |
| C | 2.12573461 | 5.58657778 | 6.88252293 |
| H | 2.12400452 | 11.06416839 | 8.68724101 |
| H | 2.44321198 | 4.68213422 | 7.43350173 |
| N | 1.82805276 | 12.73897695 | 7.45740855 |
| N | 2.20655843 | 6.76942988 | 7.38329202 |
| C | 0.92087084 | 14.06417727 | 12.29850969 |
| C | 0.64255617 | 4.90010398 | 2.92273156 |
| C | 2.76672326 | 10.96286271 | 3.72801261 |
| C | 3.23124569 | 7.72722706 | 11.37292746 |
| C | 0.76516643 | 14.74454865 | 11.08090380 |
| C | 1.06141523 | 3.83963936 | 3.73152581 |
| C | 2.41663129 | 10.15060488 | 4.81706106 |
| C | 3.36604528 | 8.64371015 | 10.32387512 |
| C | 1.03116494 | 14.12198740 | 9.87258232 |
| C | 1.55151552 | 4.05592127 | 5.01619682 |
| C | 2.09511039 | 10.68674440 | 6.05760495 |
| C | 3.06075260 | 8.28747055 | 9.01987881 |
| C | 1.47411011 | 12.78733027 | 9.83671816 |
| C | 1.61010790 | 5.35552428 | 5.53880726 |
| C | 2.14582782 | 12.07663665 | 6.26192557 |
| C | 2.60296693 | 6.99545085 | 8.70562457 |
| C | 1.59742409 | 12.09545365 | 11.04945333 |
| C | 1.15722709 | 6.42102143 | 4.74095396 |
| C | 2.51441672 | 12.88794550 | 5.17730217 |
| C | 2.49614838 | 6.06299104 | 9.75044831 |
| C | 1.32122388 | 12.72472945 | 12.25925834 |
| C | 0.68699251 | 6.19574766 | 3.45643394 |
| C | 2.81568916 | 12.34381609 | 3.93532882 |
| C | 2.80512601 | 6.43045276 | 11.05582346 |
| C | 0.67787911 | 14.76973140 | 13.60441950 |
| C | 0.18995239 | 4.64919326 | 1.51421687 |
| C | 3.02976063 | 10.36448414 | 2.37534934 |
| C | 3.50861620 | 8.14674982 | 12.79161477 |
| H | 0.43252332 | 15.78281565 | 11.09195509 |
| H | 1.01633519 | 2.82383520 | 3.34065655 |
| H | 2.38241617 | 9.06882317 | 4.68509256 |
| H | 3.70610722 | 9.65670472 | 10.53666387 |
| H | 0.90135911 | 14.64951011 | 8.92966730 |
| H | 1.88550008 | 3.20288762 | 5.60935915 |
| H | 1.77367668 | 10.01522785 | 6.85147232 |
| H | 3.16531732 | 9.00056639 | 8.20414186 |
| H | 1.94034624 | 11.06106299 | 11.03944243 |
| H | 1.16331102 | 7.42003337 | 5.17173884 |
| H | 2.57754854 | 13.95919987 | 5.34852391 |
| H | 2.10690019 | 5.06607749 | 9.55308965 |
| H | 1.44263374 | 12.17535167 | 13.19373538 |
| H | 0.33549946 | 7.03462367 | 2.85447241 |
| H | 3.10748817 | 13.00130779 | 3.11465194 |
| H | 2.67753116 | 5.70181076 | 11.85746338 |
| H | 1.07471133 | 15.79427520 | 13.59110751 |
| H | -0.33014116 | 3.68724154 | 1.42470321 |
| H | 3.57105315 | 11.06373093 | 1.72505882 |
| H | 3.14326764 | 7.41271678 | 13.51939725 |
| H | -0.40011398 | 14.86355424 | 13.81216586 |
| H | -0.47910049 | 5.44088262 | 1.15588652 |
| H | 2.09062512 | 10.10358790 | 1.86436288 |
| H | 3.05470774 | 9.12091231 | 13.02370084 |
| H | 1.11777383 | 14.22901924 | 14.45255337 |
| H | 1.04773209 | 4.61308637 | 0.82590712 |
| H | 3.61575840 | 9.43868908 | 2.44823499 |
| H | 4.58977328 | 8.26337373 | 12.97026410 |

Table 7: Coordinates of a structure of Form II with a potential energy of -6112.779867 eV

| | | | |
|---|---|---|---|
| $X_{Lattice}$ | 3.36544077 | -0.04627431 | -0.133808354 |
| $Y_{Lattice}$ | -1.7811520 | 12.338100267 | 0.158901595 |
| $Z_{Lattice}$ | -1.1576564 | -0.89328876 | 13.41072821 |
| C | 0.00962872 | -0.01381038 | 6.54162526 |
| C | 1.60173280 | 5.23304600 | 6.93303642 |
| H | 0.17051226 | 0.80452882 | 7.26808296 |
| H | 1.72243114 | 4.42308659 | 6.19003461 |
| N | -0.40022293 | -1.17818484 | 6.90577765 |
| N | 1.15781923 | 6.39618496 | 6.60679300 |
| C | 0.98033646 | 1.06863881 | 2.51211063 |
| C | 2.81780468 | 4.13001418 | 10.88960177 |
| C | -1.16655217 | -2.13495719 | 10.96113267 |
| C | 0.07519067 | 7.37775671 | 2.62995633 |
| C | 0.90214066 | 2.03060733 | 3.52326266 |
| C | 2.67730154 | 3.17314940 | 9.88100458 |
| C | -0.91103873 | -3.11381931 | 9.99650438 |
| C | 0.40864936 | 8.35022960 | 3.57697281 |
| C | 0.57704304 | 1.66895544 | 4.82669156 |
| C | 2.27740402 | 3.54024630 | 8.60015272 |
| C | -0.67953142 | -2.78612409 | 8.66489972 |
| C | 0.74834792 | 8.01373339 | 4.88273582 |
| C | 0.32152514 | 0.33189676 | 5.16175397 |
| C | 2.00136760 | 4.87897477 | 8.28819395 |
| C | -0.67909716 | -1.44526092 | 8.25766987 |
| C | 0.78016800 | 6.67036684 | 5.28074143 |
| C | 0.41859748 | -0.63829830 | 4.15301397 |
| C | 2.16165223 | 5.84471992 | 9.29300603 |
| C | -0.98655728 | -0.46108835 | 9.21473073 |
| C | 0.39714070 | 5.69193787 | 4.34529697 |
| C | 0.74830214 | -0.27228669 | 2.85633666 |
| C | 2.56908108 | 5.47318453 | 10.56548070 |
| C | -1.22120970 | -0.80111853 | 10.53946724 |
| C | 0.05508823 | 6.04134994 | 3.04611479 |
| C | 1.27866940 | 1.46945938 | 1.09625080 |
| C | 3.19941640 | 3.72033936 | 12.28268990 |
| C | -1.38974781 | -2.50764170 | 12.40127004 |
| C | -0.26247698 | 7.76157868 | 1.21520531 |
| H | 1.10436926 | 3.07489619 | 3.28314380 |
| H | 2.89385873 | 2.12880057 | 10.10565241 |
| H | -0.88694224 | -4.16117461 | 10.29850953 |
| H | 0.40861806 | 9.39959637 | 3.28093267 |
| H | 0.52232136 | 2.43054686 | 5.60734516 |
| H | 2.17820255 | 2.78173407 | 7.82063964 |
| H | -0.48600106 | -3.56585223 | 7.92828974 |
| H | 1.00085328 | 8.78915948 | 5.60600942 |
| H | 0.27107522 | -1.68103801 | 4.42157010 |
| H | 1.99851948 | 6.88847050 | 9.03809190 |
| H | -1.06955897 | 0.58060536 | 8.91106392 |
| H | 0.33725241 | 4.64778114 | 4.64661832 |
| H | 0.83168954 | -1.04240799 | 2.08730627 |
| H | 2.70151730 | 6.24041196 | 11.33055747 |
| H | -1.45811116 | -0.01675950 | 11.26091020 |
| H | -0.23732948 | 5.26117925 | 2.34060011 |
| H | 1.86317936 | 2.39713519 | 1.05940736 |
| H | 3.80947721 | 4.48348818 | 12.78208350 |
| H | -0.99722874 | -3.50720136 | 12.62628055 |
| H | 0.12640326 | 7.03761658 | 0.48709780 |
| H | 1.82720216 | 0.68736073 | 0.55661682 |
| H | 2.30713934 | 3.56750980 | 12.90904947 |
| H | -2.46395699 | -2.52504726 | 12.64817372 |
| H | 0.12915729 | 8.75462548 | 0.96161779 |
| H | 0.35123457 | 1.65456290 | 0.53318415 |
| H | 3.75272911 | 2.77339751 | 12.28194524 |
| H | -0.92689457 | -1.78845123 | 13.09006378 |
| H | -1.35308265 | 7.80134229 | 1.06011724 |

Table 8: Coordinates of a structure of Form II with a potential energy of -6112.736746 eV

| | | | |
|---|---|---|---|
| $X_{Lattice}$ | 3.36200143 | 0.1365985 | 0.2156439248 |
| $Y_{Lattice}$ | 1.8697292 | 13.08251714 | -2.0041866868 |
| $Z_{Lattice}$ | 1.64416835 | -0.5167626 | 13.257437534 |
| C | 5.39446450 | 5.35721936 | 12.45172367 |
| C | 4.04915448 | 7.00298166 | 4.96290497 |
| H | 5.29277844 | 5.18271397 | 11.36687155 |
| H | 4.36284519 | 6.30880166 | 4.16148921 |
| N | 5.78654232 | 6.49067300 | 12.92230303 |
| N | 4.07196786 | 6.68004572 | 6.20842888 |
| C | 4.32091741 | 1.90881690 | 14.75554352 |
| C | 2.66255957 | 10.82577301 | 3.62521049 |
| C | 6.75224581 | 9.77256716 | 10.40459187 |
| C | 4.86003020 | 2.82989986 | 7.76812964 |
| C | 4.48939786 | 3.15522509 | 15.37935074 |
| C | 3.00461251 | 9.82231116 | 2.71512585 |
| C | 6.69057942 | 8.47844582 | 9.87009390 |
| C | 5.00096524 | 3.99341085 | 8.53225714 |
| C | 4.85989970 | 4.28166330 | 14.65974617 |
| C | 3.48477198 | 8.58893630 | 3.14515642 |
| C | 6.37854322 | 7.38498594 | 10.66707574 |
| C | 4.77180652 | 5.24475980 | 7.98329383 |
| C | 5.04448759 | 4.20553649 | 13.27081667 |
| C | 3.58922153 | 8.31037372 | 4.51591501 |
| C | 6.11589780 | 7.53895868 | 12.03856565 |
| C | 4.39462944 | 5.38787174 | 6.63719978 |
| C | 4.84372863 | 2.96765725 | 12.64137815 |
| C | 3.21931214 | 9.30719993 | 5.43483825 |
| C | 6.23277709 | 8.82468636 | 12.58199711 |
| C | 4.28374246 | 4.22627674 | 5.85620040 |
| C | 4.49563024 | 1.83634826 | 13.37128412 |
| C | 2.76460333 | 10.54104839 | 4.99499024 |
| C | 6.53775651 | 9.91866214 | 11.77882443 |
| C | 4.50889257 | 2.97527647 | 6.41936301 |
| C | 4.00148144 | 0.68501373 | 15.56301837 |
| C | 2.24621889 | 12.18033690 | 3.13469964 |
| C | 7.01407561 | 10.96177907 | 9.52337934 |
| C | 5.05960097 | 1.47626580 | 8.39472929 |
| H | 4.32072045 | 3.23134085 | 16.45429864 |
| H | 2.90189288 | 10.01605581 | 1.64764364 |
| H | 6.89605933 | 8.31418828 | 8.81028691 |
| H | 5.28755097 | 3.91164739 | 9.58084875 |
| H | 4.97963428 | 5.24490901 | 15.15038275 |
| H | 3.76953037 | 7.84058556 | 2.40310954 |
| H | 6.37560901 | 6.39609285 | 10.21330938 |
| H | 4.86866395 | 6.14810209 | 8.58072605 |
| H | 4.96443057 | 2.89754668 | 11.55952368 |
| H | 3.28404711 | 9.07825533 | 6.49652912 |
| H | 6.08845220 | 8.94108613 | 13.65304958 |
| H | 3.96056269 | 4.29593456 | 4.81976740 |
| H | 4.35128237 | 0.88388988 | 12.85959804 |
| H | 2.48366978 | 11.30266669 | 5.72403034 |
| H | 6.61721256 | 10.90903596 | 12.23050028 |
| H | 4.37292078 | 2.08384693 | 5.80631811 |
| H | 4.92351986 | 0.21952960 | 15.94182206 |
| H | 3.12753505 | 12.81800613 | 2.96681827 |
| H | 6.07101117 | 11.36651166 | 9.12304930 |
| H | 4.55779618 | 1.39816518 | 9.37037469 |
| H | 3.38755954 | 0.92787169 | 16.43975573 |
| H | 1.71732699 | 12.11162146 | 2.17658497 |
| H | 7.63610528 | 10.69779725 | 8.65806648 |
| H | 6.12753736 | 1.27917593 | 8.58336488 |
| H | 3.48205701 | -0.07480791 | 14.96535521 |
| H | 1.60417636 | 12.70194442 | 3.85406280 |
| H | 7.50257473 | 11.77705985 | 10.07395001 |
| H | 4.69475591 | 0.66561229 | 7.75345886 |

Table 9: Coordinates of a structure of Form II with a potential energy of -6112.704336 eV

| | | | |
|---|---|---|---|
| $X_{Lattice}$ | 4.61912018 | -0.07897357 | -0.222727636 |
| $Y_{Lattice}$ | 0.08213397 | 9.8648312 | -0.3819479216 |
| $Z_{Lattice}$ | 0.48988074 | 0.31785377 | 12.041887551 |
| C | 4.35729644 | 5.23170928 | -0.23225252 |
| C | 2.35023477 | 4.87507354 | 6.23766373 |
| H | 4.57107179 | 5.43915662 | 0.82574940 |
| H | 2.60547877 | 5.55081498 | 7.06899307 |
| N | 4.95492190 | 4.28862547 | -0.87434914 |
| N | 2.89320312 | 4.98295316 | 5.07534214 |
| C | 1.41926666 | 7.91680291 | -1.82336661 |
| C | -0.54125268 | 1.93092788 | 7.38341990 |
| C | 7.85722295 | 1.73169001 | 0.88952281 |
| C | 5.72565421 | 7.97371555 | 4.02779538 |
| C | 1.93886827 | 6.88607116 | -2.61883533 |
| C | -0.04980509 | 2.87510543 | 8.29335380 |
| C | 7.34868705 | 2.81109841 | 1.62494760 |
| C | 5.17752099 | 7.08084952 | 3.10040159 |
| C | 2.89010571 | 5.99686709 | -2.13226686 |
| C | 0.88373722 | 3.82643800 | 7.90029388 |
| C | 6.40008437 | 3.67571699 | 1.08663755 |
| C | 4.25897269 | 6.11236373 | 3.48743767 |
| C | 3.35857651 | 6.11535860 | -0.81499086 |
| C | 1.36017259 | 3.86650372 | 6.58056225 |
| C | 5.91381556 | 3.48895211 | -0.22183884 |
| C | 3.83939413 | 5.99060946 | 4.81896328 |
| C | 2.82588184 | 7.13481855 | -0.00769147 |
| C | 0.85173373 | 2.93942358 | 5.65534057 |
| C | 6.43929600 | 2.41933585 | -0.96321046 |
| C | 4.40581849 | 6.87133788 | 5.76181609 |
| C | 1.87648336 | 8.01935606 | -0.50236069 |
| C | -0.08033874 | 1.99075094 | 6.05719471 |
| C | 7.38639286 | 1.56017184 | -0.41896686 |
| C | 5.32260805 | 7.83997669 | 5.36517288 |
| C | 0.40187540 | 8.87783417 | -2.35295772 |
| C | -1.53309836 | 0.89539841 | 7.81718423 |
| C | 8.87423177 | 0.79560058 | 1.46998643 |
| C | 6.71220571 | 9.02073736 | 3.60604620 |
| H | 1.58110870 | 6.79205327 | -3.64553899 |
| H | -0.38927103 | 2.86582005 | 9.32989005 |
| H | 7.69519640 | 2.98368166 | 2.64648864 |
| H | 5.47505608 | 7.15659406 | 2.05278492 |
| H | 3.28384805 | 5.19648262 | -2.75792923 |
| H | 1.25848961 | 4.53511370 | 8.64111896 |
| H | 6.04599546 | 4.49654995 | 1.70897925 |
| H | 3.82420394 | 5.42283217 | 2.76490030 |
| H | 3.17103482 | 7.22931393 | 1.02293127 |
| H | 1.20427419 | 2.97847928 | 4.62528762 |
| H | 6.08099492 | 2.28147816 | -1.98247392 |
| H | 4.13764323 | 6.80518397 | 6.81593381 |
| H | 1.48523193 | 8.81168884 | 0.13617947 |
| H | -0.45993389 | 1.26698185 | 5.33499606 |
| H | 7.77063083 | 0.73429158 | -1.01808968 |
| H | 5.73719023 | 8.52092906 | 6.11027060 |
| H | 0.67481449 | 9.91647208 | -2.12313962 |
| H | -2.55861033 | 1.21316089 | 7.57882237 |
| H | 9.84993116 | 0.92561968 | 0.98023374 |
| H | 6.60874926 | 9.26015100 | 2.54124705 |
| H | 0.28500196 | 8.78642923 | -3.43802076 |
| H | -1.35924504 | -0.06307987 | 7.31099158 |
| H | 8.57687746 | -0.25356372 | 1.33368115 |
| H | 7.74449824 | 8.67688847 | 3.76574250 |
| H | -0.58056966 | 8.69186711 | -1.89598855 |
| H | -1.48605201 | 0.72744385 | 8.89877258 |
| H | 9.01678685 | 0.97255271 | 2.54175751 |
| H | 6.58186354 | 9.94885006 | 4.17646534 |

Table 10: Coordinates of a structure of Form II with a potential energy of -6112.686329 eV
